# Supplementary material for: Size-effects of metamaterial beams subjected to pure bending: on boundary conditions and parameter identification in the relaxed micromorphic model
Source: arXiv:2210.17117 source file (2023-03-28)
Supplement: Supplementary file 1 [file appendixA.tex]

\sect{Appendix}
\label{app:Nedelec_shape_functions}
\ssect{Construction of N\'ed\'elec shape functions in the parameter space}
The parameter elements are defined in the natural coordinates $\Bxi = (\xi,\eta)^T$. Triangular element is defined by the domain $\B_e^\triangle = \{0 \le \xi \le 1, 0 \le \eta \le 1 - \xi\}$ while quadrilateral element has the domain $\B_e^\square = \{-1 \le \xi \le 1, -1 \le \eta \le 1\}$. 
\sssect{\hspace{-5mm}. First-order triangular element NT1 \\} 
N\'ed\'elec shape functions general form for $k=1$ following Equation \ref{eq:t:shape_functions_form_t} reads
\begin{equation}
\bv_I = \left[\begin{array}{c}
a_1 - a_3 \eta \\ 
a_2 + a_3 \xi
\end{array}\right]\,.
\end{equation}
The following table shows the calculations of the dofs  in Equation \ref{eq:t:edge_dof}: 
\begin{center}
\begin{table}[ht]
\begin{tabular}{|c|c|c|c|c|}
\cline{1-5}
$I$ &  $q_j$ & $\tau_i$ &  $\xi-\eta$ coloration & $m_{ij}$   \\  \cline{1-5}
1 & $1$ & $(1,0)^T$ & $\eta = 0$ & $a_1$ \\
\cline{1-5}
2 & $1$ & $(\frac{1}{\sqrt{2}},-\frac{1}{\sqrt{2}})^T$ & $ \eta = 1 - \xi$ & $a_1-a_2-a_3$ \\
\cline{1-5}
3 & $1$ & $(0,1)^T$ & $\xi  =0$ & $a_2$ \\
\cline{1-5}
\end{tabular}
\end{table}
\end{center}
and the system of equation, which is obtained be setting one dof to one and the other to zeros, leads to the following vectorial shape function demonstrated in Figure \ref{Fig:shape_function_NT1}
\begin{equation} 
\bv_1 =  \left( \begin{array}{c}
\eta \\ 
- \xi
\end{array} \right) \,,
\bv_2 =  \left( \begin{array}{c}
\eta \\
 1 - \xi
\end{array} \right)\,, \quad
\bv_3 =  \left( \begin{array}{c}
1 - \eta \\ 
\xi
\end{array} \right) \,.
\end{equation}
\begin{figure}[ht]
     \begin{subfigure}[b]{0.32\textwidth}
         \centering
         \includegraphics[width=\textwidth]{figures/NT1_V1.pdf}
        \caption{$\bv_1$}
     \end{subfigure}
     \begin{subfigure}[b]{0.32\textwidth}
         \centering
         \includegraphics[width=\textwidth]{figures/NT1_V2.pdf}
  \caption{$\bv_2$}
     \end{subfigure}
          \begin{subfigure}[b]{0.32\textwidth}
         \centering
         \includegraphics[width=\textwidth]{figures/NT1_V3.pdf}
  \caption{$\bv_3$}
     \end{subfigure}
        \caption{Tangential-conforming vectorial shape functions of NT1 element. Blue circles indicate the position where the dofs are defined. }
        \label{Fig:shape_function_NT1}
\end{figure}

\sssect{\hspace{-5mm}. Second-order triangular element NT2 \\} 
The general form of the shape functions for $k=2$ following Equation \ref{eq:t:shape_functions_form_t} reads
\begin{equation}
\bv_I =  \left( \begin{array}{c}
a_1 + a_2 \xi + a_3 \eta - a_7 \eta^2 - a_8 \xi\eta \\
a_4 + a_5 \xi + a_6 \eta + a_7 \eta\xi + a_8 \xi^2
\end{array} \right) \,.
\end{equation}
The inner and outer dofs are calculated according to Equations \ref{eq:t:edge_dof} and \ref{eq:t:inner_dof_t} in the following table: 
\begin{center}
\begin{table}[ht]
\begin{tabular}{|c|c|c|c|c|}
\cline{1-5}
$I$ &  $q_j/\bq_i$ & $\tau_i$ &  $\xi-\eta$ coloration & $m_{ij}/m_i$   \\  \cline{1-5}
1 & $\xi$ & $(\frac{1}{\sqrt{2}},-\frac{1}{\sqrt{2}})^T$ & $\eta = 1 - \xi$ & $\frac{1}{6}(3 a_1 + 2 a_2 + a_3 - 3 a_4 - 2 a_5 - a_6 - a_7 - 2 a_8)$ \\
\cline{1-5}
2 & $ \eta$ & $(\frac{1}{\sqrt{2}},-\frac{1}{\sqrt{2}})^T$ & $\xi = 1 - \eta$ & $\frac{1}{6}  (3 a_1 + a_2 + 2 a_3 - 3 a_4 - a_5 - 2 a_6 - 2 a_7 - a_8)$\\
\cline{1-5}
3 & $ \eta$ & $(0,1)^T$ & $\xi = 0$ & $\frac{1}{6} (3a_4 + 2 a_6)$ \\
\cline{1-5}
4& $ (1 - \eta)$ & $(0,1)^T$ & $\xi = 0$ & $\frac{1}{6} ( 3a_4 + a_6)$ \\
\cline{1-5}
5& $ (1 - \xi)$ & $(1,0)^T$ & $\eta = 0$ & $\frac{1}{6} (3a_1 + a_2)$  \\
\cline{1-5}
6& $\xi$ & $(1,0)^T$ & $\eta = 0$ & $\frac{1}{6} (3a_1 + 2a_2)$ \\
\cline{1-5}
7& $(0,1)^T$ &-& - & $\frac{1}{24} (12 a_4 + 4 a_5 + 4 a_6 + a_7 + 2 a_8)$ \\
\cline{1-5}
8& $(1,0)^T$ &-& - & $\frac{1}{24} (12 a_1 + 4 a_2 + 4 a_3 - 2 a_7 - a_8)$  \\
\cline{1-5}
\end{tabular}
\end{table}
\end{center}
and the resulting shape functions demostrated in Figure \ref{Fig:shape_function_NT2} are obtained by setting one dof to one and the rest to zeros as
\begin{equation}
\begin{aligned}
\bv_1&= 2 \left( \begin{array}{c} 
-\eta + 4 \eta \xi \\
 2 \xi - 4 \xi^2 
 \end{array} \right)\,,\quad  \bv_2 =2 \left( \begin{array}{c} 
-2 \eta + 4 \eta^2 \\
\xi - 4 \eta \xi
 \end{array} \right)\,,\quad   \bv_3 = 2\left( \begin{array}{c} 
-2 \eta + 4 \eta^2 \\
 -1 + 3 \eta + \xi - 4 \eta \xi
 \end{array} \right), \\
 \bv_4&= 2\left( \begin{array}{c} 
3 \eta - 4 \eta^2 - 4 \eta \xi \\
 2 - 3 \eta - 6 \xi + 4 \eta \xi + 4 \xi^2
 \end{array} \right)\,,\quad   \bv_5 = 2\left( \begin{array}{c} 
2 - 6 \eta + 4 \eta^2 - 3 \xi + 4 \eta \xi \\
 3 \xi - 4 \eta \xi - 4 \xi^2
 \end{array} \right), \\
 \bv_6&= 2\left( \begin{array}{c} 
-1 + \eta + 3 \xi - 4 \eta \xi \\
 -2 \xi + 4 \xi^2
 \end{array} \right) \,,\quad 
  \bv_7= 2\left( \begin{array}{c} 
-4 \eta + 4 \eta^2 + 8 \eta \xi \\
8 \xi - 4 \eta \xi - 8 \xi^2
 \end{array} \right), \\
  \bv_8 &= 2\left( \begin{array}{c} 
8 \eta - 8 \eta^2 - 4 \eta \xi \\
-4 \xi + 8 \eta \xi +  4 \xi^2
 \end{array} \right)\,.
 \end{aligned}
\end{equation}

\begin{figure}[ht]
     \begin{subfigure}[b]{0.32\textwidth}
         \centering
         \includegraphics[width=\textwidth]{figures/NT2_V1.pdf}
        \caption{$\bv_1$}
     \end{subfigure}
     \begin{subfigure}[b]{0.32\textwidth}
         \centering
         \includegraphics[width=\textwidth]{figures/NT2_V2.pdf}
  \caption{$\bv_2$}
     \end{subfigure}
          \begin{subfigure}[b]{0.32\textwidth}
         \centering
         \includegraphics[width=\textwidth]{figures/NT2_V3.pdf}
  \caption{$\bv_3$}
     \end{subfigure}
          \begin{subfigure}[b]{0.32\textwidth}
         \centering
         \includegraphics[width=\textwidth]{figures/NT2_V4.pdf}
        \caption{$\bv_4$}
     \end{subfigure}
     \begin{subfigure}[b]{0.32\textwidth}
         \centering
         \includegraphics[width=\textwidth]{figures/NT2_V5.pdf}
  \caption{$\bv_5$}
     \end{subfigure}
          \begin{subfigure}[b]{0.32\textwidth}
         \centering
         \includegraphics[width=\textwidth]{figures/NT2_V6.pdf}
  \caption{$\bv_6$}
     \end{subfigure}
          \begin{subfigure}[b]{0.32\textwidth}
         \centering
         \includegraphics[width=\textwidth]{figures/NT2_V7.pdf}
        \caption{$\bv_7$}
     \end{subfigure}
  \begin{subfigure}[b]{0.32\textwidth}
         \centering
         \includegraphics[width=\textwidth]{figures/NT2_V8.pdf}
        \caption{$\bv_8$}
     \end{subfigure}
       \caption{Tangential-conforming vectorial shape functions of NT2 element. Blue circles indicate the position where the dofs are defined. }
        \label{Fig:shape_function_NT2}
\end{figure}

\sssect{\hspace{-5mm}. First-order quadrilateral element NQ1 \\} 
The general form of the vectorial shape function of N\'ed\'elec type for the quadrilateral element following Equation  \ref{eq:t:shape_functions_form_q} reads 
\begin{equation}
\bv =  \left( \begin{array}{c}
a_1 + a_2 \eta  \\ a_3 + a_4 \xi
\end{array} \right) \,.
\end{equation}
We calculate the edge dofs using Equation \ref{eq:t:edge_dof}  in the following table:
\begin{center}
\begin{table}[ht]
\begin{tabular}{|c|c|c|c|c|}
\cline{1-5}
$I$ &  $q_j$ & $\tau_i$ &  $\xi-\eta$ coloration & $m_{ij}$   \\  \cline{1-5}
1 & $1$ & $(1,0)^T$ & $\eta = -1$ & $2(a_1 - a_2)$ \\
\cline{1-5}
2 & $1$ & $(0,1)^T$ & $\xi = 1$ & $2(a_3 + a_4)$ \\
\cline{1-5}
3 & $1$ & $(1,0)^T$ & $\eta = 1$ & $2(a_1 + a_2)$ \\
\cline{1-5}
4 & $1$ & $(0,1)^T$ & $\xi = -1$ & $2(a_3 - a_4)$ \\
\cline{1-5}
\end{tabular}
\end{table}
\end{center}
We solve the system of equations obtained by setting one dof to one while the other to zeros leading to the following shape functions demonstrated in Figure \ref{Fig:shape_function_NQ1}
\begin{equation}
\begin{aligned}
\bv_{1} =&  \left( \begin{array}{c}
(-\eta + 1)/4 \\
0 
\end{array} \right) \,, \quad 
\bv_{2} =  \left( \begin{array}{c}
0 \\
 (\xi + 1)/4 
\end{array} \right) \,, \\
\bv_{3} =&  \left( \begin{array}{c}
(\eta + 1)/4 \\
0
\end{array} \right) \,, \quad 
\bv_{4} =  \left( \begin{array}{c}
0 \\
 (-\xi + 1)/4
\end{array}\right)\,.
\end{aligned}
\end{equation}

\begin{figure}[ht]
    \centering
     \begin{subfigure}[b]{0.33\textwidth}
         \centering
         \includegraphics[width=\textwidth]{figures/NQ1_V1.pdf}
        \caption{$\bv_1$}
     \end{subfigure}
     \begin{subfigure}[b]{0.33\textwidth}
         \centering
         \includegraphics[width=\textwidth]{figures/NQ1_V2.pdf}
  \caption{$\bv_2$}
     \end{subfigure}
          \begin{subfigure}[b]{0.33\textwidth}
         \centering
         \includegraphics[width=\textwidth]{figures/NQ1_V3.pdf}
  \caption{$\bv_3$}
     \end{subfigure}
          \begin{subfigure}[b]{0.33\textwidth}
         \centering
         \includegraphics[width=\textwidth]{figures/NQ1_V4.pdf}
        \caption{$\bv_4$}
     \end{subfigure}
       \caption{Tangential-conforming vectorial shape functions of NQ1 element. Blue circles indicate the position where the dofs are defined. }
        \label{Fig:shape_function_NQ1}
\end{figure}

\sssect{\hspace{-5mm}. Second-order quadrilateral element NQ2 \\} 
Second-order N\'ed\'elec tangential-conforming  basis functions for quadrilateral element has the following general form 
\begin{equation}
\bv =  \left( \begin{array}{c}
a_1 + a_2 \xi + a_3 \eta + a_4 \xi \eta + a_5 \eta^2 + 
 a_6 \xi \eta^2 \\ a_7 + a_8 \xi + a_9 \eta + 
 a_{10} \xi \eta + a_{11} \xi^2 + a_{12} \eta \xi^2
\end{array} \right) \,.
\end{equation}
The edge and inner dofs are calculated according to Equations  \ref{eq:t:edge_dof} and \ref{eq:t:inner_dof_q}  in the following table:
\begin{center}
\begin{table}[ht]
\begin{tabular}{|c|c|c|c|c|}
\cline{1-5}
$I$ &  $q_j/\bq_i$ & $t_i$ &  $\xi-\eta$ coloration & $m_{ij}/m_i$   \\  \cline{1-5}
1 & $\frac{1}{2}  (1 - \xi)$ & $(1,0)^T$ & $\eta = -1$ & $\frac{1}{3} \, (3a_1 - a_2 - 3a_3 + a_4 + 3a_5 - a_6)$ \\
\cline{1-5}
2 & $\frac{1}{2}  (1+ \xi)$ & $(1,0)^T$ & $\eta = -1$ & $\frac{1}{3}  \, (3a_1 + a_2 - 3a_3 - a_4 + 3a_5 + a_6)$ \\
\cline{1-5}
3 & $\frac{1}{2}  (1 - \eta)$ & $(0,1)^T$ & $\xi = 1$ & $\frac{1}{3}  \, (-a_{10} +3a_{11} - a_{12} + 3a_7 + 3a_8 - a_9)$ \\
\cline{1-5}
4 & $\frac{1}{2}  (1 + \eta)$ & $(0,1)^T$ & $\xi = 1$ & $\frac{1}{3}  \, (a_{10} +3a_{11} + a_{12} + 3a_7 + 3a_8 + a_9)$ \\
\cline{1-5}
5 & $\frac{1}{2}  (1+ \xi)$ & $(1,0)^T$ & $\eta = 1$ & $\frac{1}{3} \,(3a_1 + a_2 + 3a_3 + a_4 + 3a_5 + a_6)$ \\
\cline{1-5}
6 & $\frac{1}{2}  (1 - \xi)$ & $(1,0)^T$ & $\eta = 1$ & $\frac{1}{3} \,(3a_1 - a_2 + 3a_3 - a_4 + 3a_5 - a_6)$ \\
\cline{1-5}
7 & $\frac{1}{2}  (1 + \eta)$ & $(0,1)^T$ & $\xi = -1$ & $\frac{1}{3} \,( -a10 + a11 + a12 + a7 - a8 + a9/3)$ \\
\cline{1-5}
8 & $\frac{1}{2}  (1 - \eta)$ & $(0,1)^T$ & $\xi = -1$ & $\frac{1}{3} \,( a10 + a11 - a12 + a7 - a8 - a9/3)$ \\
\cline{1-5}
9 &  $(\frac{1}{2}  (1+ \xi),0)^T$& - & -& $\frac{2}{9} (9 a_1 + 3 a_2 + 3 a_5 + a_6)$ \\
\cline{1-5}
10 &  $(\frac{1}{2}  (1- \xi),0)^T$& - & -& $\frac{2}{9} (9 a_1 - 3 a_2 + 3 a_5 - a_6)$ \\
\cline{1-5}
11 &  $(0,\frac{1}{2}  (1 + \eta))^T$& - & -& $\frac{2}{9} (3 a_{11} + a_{12} + 9 a_7 + 3 a_9)$ \\
\cline{1-5}
12 &  $(0,\frac{1}{2}  (1 - \eta))^T$& - & -& $\frac{2}{9} (3 a_{11} - a_{12} + 9 a_7 - 3 a_9)$ \\
\cline{1-5}
\end{tabular}
\end{table}
\end{center}

The N\'ed\'elec  basis functions ($\bv_I$) demonstrated in Figure  \ref{Fig:shape_function_NQ2}  are obtained by enforcing a value of one for the related dof and zeros for the rest: 

\begin{equation}
\begin{aligned}
\bv_1 &= \left( \begin{array}{c} 
-1/8 - \eta/4 + 3 \eta^2 /8 + 3 \xi/8 +  3 \eta \xi/4 - 9 \eta^2 \xi/8 \\
0
 \end{array} \right), \\
  \bv_2 &= \left( \begin{array}{c} 
-1/8 - \eta/4 + 3 \eta^2 /8 - 3 \xi/8 -  3 \eta \xi/4 + 9 \eta^2 \xi/8 \\
0
 \end{array} \right), \\
  \bv_3& = \left( \begin{array}{c} 
0 \\
- 1/8 + 3 \eta/8 + \xi/4 - 3 \eta \xi/4 +  3 \xi^2/8 - 9 \eta \xi^2/8
 \end{array} \right), \\
 \bv_4 &= \left( \begin{array}{c} 
0 \\
- 1/8 - 3 \eta/8 + \xi/4 + 3 \eta \xi/4 +  3 \xi^2/8 + 9 \eta \xi^2/8
 \end{array} \right), \\
  \bv_5 &= \left( \begin{array}{c} 
-1/8 + \eta/4 + 3 \eta^2/8 - 3 \xi/8 +  3 \eta \xi/4 + 9 \eta^2 \xi/8 \\
0
 \end{array} \right), \\
 \bv_6 &= \left( \begin{array}{c} 
-1/8+ \eta/4 + 3 \eta^2/8 +  3 \xi/8 - 3 \eta \xi/4 - 9 \eta^2 \xi/8 \\
0
 \end{array} \right), \\
  \bv_7 &= \left( \begin{array}{c} 
0 \\
-1/8 - 3 \eta/8 - \xi/4 - 3 \eta \xi/4 +  3 \xi^2/8 + 9 \eta \xi^2/8
 \end{array} \right), \\
  \bv_8 &= \left( \begin{array}{c} 
0 \\
-1/8 + 3 \eta/8 - \xi/4 + 3 \eta \xi/4 +  3 \xi^2/8 - 9 \eta \xi^2/8
 \end{array} \right)\,.
  \\
  \bv_9 &= \left( \begin{array}{c} 
3/8 - 3 \eta^2/8 + 9 \xi/8 - 9 \eta^2 \xi/8 \\
0
 \end{array} \right)\,, \quad  \bv_{10} = \left( \begin{array}{c} 
3/8 - 3 \eta^2/8 - 9 \xi/8 + 9 \eta^2 \xi/8 \\
0
 \end{array} \right)\,, \\
   \bv_{11} &= \left( \begin{array}{c} 
0 \\
3/8 +9 \eta/8 - 3 \xi^2/8 - 9 \eta \xi^2/8
 \end{array} \right)\,, \quad  \bv_{12} = \left( \begin{array}{c} 
0 \\
3/8 -9 \eta/8 - 3 \xi^2/8 + 9 \eta \xi^2/8
 \end{array} \right)\,.
 \end{aligned}
\end{equation}

\begin{figure}[ht]
     \begin{subfigure}[b]{0.32\textwidth}
         \centering
         \includegraphics[width=\textwidth]{figures/NQ2_V1.pdf}
        \caption{$\bv_1$}
     \end{subfigure}
     \begin{subfigure}[b]{0.32\textwidth}
         \centering
         \includegraphics[width=\textwidth]{figures/NQ2_V2.pdf}
  \caption{$\bv_2$}
     \end{subfigure}
          \begin{subfigure}[b]{0.32\textwidth}
         \centering
         \includegraphics[width=\textwidth]{figures/NQ2_V3.pdf}
  \caption{$\bv_3$}
     \end{subfigure}
          \begin{subfigure}[b]{0.32\textwidth}
         \centering
         \includegraphics[width=\textwidth]{figures/NQ2_V4.pdf}
        \caption{$\bv_4$}
     \end{subfigure}
       \begin{subfigure}[b]{0.32\textwidth}
         \centering
         \includegraphics[width=\textwidth]{figures/NQ2_V5.pdf}
        \caption{$\bv_5$}
     \end{subfigure}
     \begin{subfigure}[b]{0.32\textwidth}
         \centering
         \includegraphics[width=\textwidth]{figures/NQ2_V6.pdf}
  \caption{$\bv_6$}
     \end{subfigure}
          \begin{subfigure}[b]{0.32\textwidth}
         \centering
         \includegraphics[width=\textwidth]{figures/NQ2_V7.pdf}
  \caption{$\bv_7$}
     \end{subfigure}
          \begin{subfigure}[b]{0.32\textwidth}
         \centering
         \includegraphics[width=\textwidth]{figures/NQ2_V8.pdf}
        \caption{$\bv_8$}
     \end{subfigure}
        \begin{subfigure}[b]{0.32\textwidth}
         \centering
         \includegraphics[width=\textwidth]{figures/NQ2_V9.pdf}
        \caption{$\bv_9$}
     \end{subfigure}
     \begin{subfigure}[b]{0.32\textwidth}
         \centering
         \includegraphics[width=\textwidth]{figures/NQ2_V10.pdf}
  \caption{$\bv_{10}$}
     \end{subfigure}
          \begin{subfigure}[b]{0.32\textwidth}
         \centering
         \includegraphics[width=\textwidth]{figures/NQ2_V11.pdf}
  \caption{$\bv_{11}$}
     \end{subfigure}
          \begin{subfigure}[b]{0.32\textwidth}
         \centering
         \includegraphics[width=\textwidth]{figures/NQ2_V12.pdf}
        \caption{$\bv_{12}$}
     \end{subfigure}
       \caption{Tangential-conforming vectorial shape functions of NQ2 element.  Blue circles indicate the position where the dofs are defined. }
        \label{Fig:shape_function_NQ2}
\end{figure}
